# Supplementary material for: Improving IoT Analytics through Selective Edge Execution
Source: arXiv:2003.03588 source file (2020-03-07)
Supplement: Supplementary file 1 [file Appendix_V4.tex]

\section{Appendix: Proof of Theorem 1} \label{sec:SM}

We drop bold typeface notation here; use subscript $i=1,\ldots,t$ to denote the $i$th slot; and $n$ for the $n$th component of a vector. We will be using the following Lagrangians:
\begin{align}
&L(y_t, \mu_t, \delta_t, \epsilon_t)	= f(y_t) + y_t^\top \epsilon_t + \mu_t^\top\big(g(y_t) + \delta_t(y_t)\big) \label{eq:L1} \\
&L(y_t, \mu_t, \delta_t)	= f(y_t) + \mu_t^\top\big(g(y_t) + \delta_t(y_t)\big) \\
&L(y_t, \mu_t)	= f(y_t) + \mu_t^\top g(y_t) \label{eq:L3}
\end{align}
\eqref{eq:L1} is the Lagrangian used in the subgradient method; and unless stated otherwise, we will use below $y_t\in\argmin_{y\in\mathcal{Y}} L(y, \mu_t, \delta_t, \epsilon_t)$. We denote with $V(\mu, \delta_t)$ and $V(\mu, \delta_t, \epsilon_t)$ the respective dual functions. We first bound the distance of $\mu_{t+1}$ from vector $\theta\in \mathbf R^{N+1}$, i.e., $\norm{ \mu_{t+1}-\theta }_{2}^2=$
\begin{align}
	&\norm{ [\mu_t+a\big( g(y_t)+\delta_t(y_t)\big) ]^+ -\theta }_{2}^2 \leq \nonumber\\
	&\norm{ \mu_t+a\big( g(y_t)+\delta_t(y_t)\big)  -\theta }_{2}^2=\nonumber \\
	&\norm{ \mu_t-\theta }_{2}^2 +a^2\norm{ g(y_t)+\delta_t(y_t) }_2^2+ \nonumber \\ &2a(\mu_t-\theta)^\top\big( g(y_t)+\delta_t(y_t)\big)\leq \nonumber \\
	&\norm{ \mu_t-\theta }_{2}^2 \!+\!a^2\norm{ g(y_t)}_{2}^2\!+\! a^2\norm{ \delta_t(y_t)}_{2}^2 \!+\! 2a^2\delta_t(y_t)^\top g(y_t)+ \notag\\ 
	&2a (\mu_t\!-\!\theta)^\top\big(g(y_t)\!+\!\delta_t(y_t)\big) \label{eq:15} 
\end{align}

Next, we bound the difference of $L(y_t, \mu_t, \delta_t, \epsilon_t)$ from $V(\mu_t)$. We define $\hat y_t\in\argmin_{y\in\mathcal{Y}} L(y, \mu_t)$, which is different from $y_t$. Then, we can write:
\begin{align}
L(y_t, \mu_t, \delta_t, \epsilon_t)&=L(\hat y_t, \mu_t) +  L(y_t, \mu_t, \delta_t, \epsilon_t)-L(\hat y_t, \mu_t)\notag\\
&\leq V(\mu_t) + A_t(\hat y_t, y_t) \label{eq:19}
\end{align}
where we defined 
\begin{equation}
A_t(\hat y_t, y_t)=f(y_t)-f(\hat y_t) + y_t^\top\epsilon_t + \mu_t^\top\big( g(y_t)-g(\hat y_t)+\delta_t(y_t) \big), \notag
\end{equation}
and used $L(\hat y_t, \mu_t)=V(\mu_t)$. By Assumption 1, it holds that $\lim_{t\rightarrow \infty}L(\cdot,\mu_t, \delta_t, \epsilon_t)=L(\cdot, \mu_t)$, and given that these are continuous convex functions, this yields $\lim_{t\rightarrow \infty}A_t(\hat y_t, y_t)=0$. Also, we can upper bound $A_t(\cdot)$ for every $t$, since the objective and constraint functions are upper bounded (all their components), and also the dual vector is bounded for any $t$ (as we will prove in the sequel). Therefore, it also holds that $\lim_{t\rightarrow \infty}\frac{1}{t}\sum_{i=1}^tA_i(\hat y_i, y_i)=0$.

\underline{\textbf{(i) Optimality Gap}}. Using \eqref{eq:19}, and defining $\bar y_t=\frac{1}{t}\sum_{i=1}^ty_i$, we can write:
\begin{align}
	V(\mu^*)\!&\geq\! \frac{1}{t}\sum_{i=1}^tV(\mu_i)\!\geq\! \frac{1}{t}\sum_{i=1}^t \big(L(y_i,\mu_i, \delta_i, \epsilon_i)\!-\!A_i(\hat y_i, y_i\big)\! \nonumber \\
	&=\!\frac{1}{t}\sum_{i=1}^t\Big( f(y_i)\!+\!y_i^\top\epsilon_i\!+\!\mu_i^\top\big(g(y_i)\!+\!\delta_i(y_i)\big) -\!A_i(\hat y_i, y_i) \Big) \nonumber \\
	&\geq f(\bar y_t)+\frac{1}{t}\sum_{i=1}^ty_i^\top\epsilon_i \nonumber \\
	&+ \frac{1}{t}\sum_{i=1}^t\Big( \mu_i^\top\big( g(y_i)+\delta_i(y_i) \big) - A_i(\hat y_i, y_i) \Big),
\end{align}
where the last inequality follows from Jensen's rule. Hence:
\begin{align}
	&f(\bar y_t)-V(\mu^*) \leq \nonumber \\
	&-\frac{1}{t}\sum_{i=1}^ty_i^\top\epsilon_i -\frac{1}{t}\sum_{i=1}^t \Big( \mu_i^\top\big( g(y_i)+\delta_i(y_i)\big) - A_i(\hat y_i, y_i) \Big) \label{eq:21}
\end{align}
Now, let $\theta=0$ in \eqref{eq:15}, we get:
\begin{align}
	\norm{ \mu_{t+1} }_2^2 &\leq \norm{ \mu_t }_2^2 + a^2 \norm{ g(y_t) }_2^2 + a^2 \norm{\delta_t(y_t)}_2^2+ \nonumber \\
	&2a^2\delta_t(y_t)^\top g(y_t) + 2a \mu_t^\top \big( g(y_t)+\delta_t(y_t) \big),
\end{align}
and using \eqref{eq:var} and the Cauchy-Swartz inequality:
\begin{align}
	\norm{ \mu_{t+1} }_2^2 &\leq \norm{ \mu_t }_2^2 + a^2 \sigma_g^2 + a^2\sigma_{\delta_t}^2 + \nonumber \\
	&2a^2\sigma_{g}\sigma_{\delta_t} + 2a \mu_t^\top \big( g(y_t)+\delta_t(y_t) \big).
\end{align}
Applying it for all $t$ and summing, we obtain:
\begin{align}
	\norm{ \mu_{t+1} }_2^2 &\leq \norm{ \mu_1 }_2^2 + a^2t\sigma_g^2+ a^2\sum_{i=1}^t\sigma_{\delta_t}^2 + \nonumber \\
	&2a^2\sigma_g\sum_{i=1}^t\sigma_{\delta_t} + 2a\sum_{i=1}^t \mu_i^\top \big( g(y_i)+\delta_i(y_i) \big), \nonumber
\end{align}
which, if we drop the non-negative term $\norm{ \mu_{t+1} }_2^2$, divide by $2at$, and rearrange terms, yields:
\begin{align}
	-\frac{1}{t}\sum_{i=1}^t\mu_i^\top\big( g(y_i)+\delta_i(y_i) \big) &\leq \frac{ \norm{\mu_1}_2^2 }{2at} + \frac{a\sigma_g^2}{2} + \nonumber \\
	&\frac{a}{2t}\sum_{i=1}^t\sigma_{\delta_i}^2 +\frac{a\sigma_g}{t}\sum_{i=1}^t\sigma_{\delta_i}. \label{eq:23}
\end{align}
Setting $\mu_1=0$, using the fact that $V(\mu^*)=f^*$, and combining \eqref{eq:21} with \eqref{eq:23}, we obtain:
\begin{align}
	f(\bar y_t)-f^* &\leq -\frac{1}{t}\sum_{i=1}^ty_i^\top\epsilon_i + \frac{1}{t}\sum_{i=1}^tA_i(\hat y_i, y_i)+ \frac{a\sigma_g^2}{2}+ \nonumber \\
	&\frac{a}{2t}\sum_{i=1}^t\sigma_{\delta_i}^2+\frac{a\sigma_g}{t}\sum_{i=1}^t\sigma_{\delta_i}
\end{align}
All sums have diminishing terms and divided by $t$, hence converge to $0$. Thus, we obtained the first part of the theorem.
%: 
%\begin{equation}
%	\lim_{k\rightarrow \infty}f(\bar y_t)-f^*\leq \frac{a\sigma_g^2}{2},
%\end{equation}
%which can be made arbitrarily small by selecting accordingly the step size $\alpha$.

\underline{\textbf{(ii) Constraint Violation}}. If we apply recursively the following inequality:
\begin{align}
\mu_{t+1}&=\Big[ \mu_t + a\big( g(y_t)+\delta_t(y_t) \big) \Big]^+ \nonumber \\
&\succeq \mu_t + a\big( g(y_t)+\delta_t(y_t) \big),\,\,\,\,\text{we obtain:} \nonumber \\
\mu_{t+1}&\succeq \mu_1 + a\sum_{i=1}^t\big( g(y_i)+\delta_i(y_i) \big).
\end{align}
Dropping $\mu_1=0$, dividing by $at$, and using Jensen's inequality for $g(\cdot)$, we get:
\begin{align}
	g(\bar y_t) + \frac{1}{t}\sum_{i=1}^t\delta_i(y_i) \preceq \frac{\mu_{t+1}}{at}. \label{eq:constraint-bound}
\end{align}
We wish to prove that $\lim_{t\rightarrow\infty}g(\bar y_t)\preceq 0$. We already know that the second term in the LHS converges to zero, hence it suffices to prove that all components of vector $\mu_{t+1}$ are bounded for every $t$. This will ensure that the RHS converges to 0. We will be using the following assumption. 
%\vspace{-2mm}
\begin{assumption}
	There exists a Slater vector $y^s\in\mathcal{Y}$ such that $g( y^s)+\delta_t(y^s)\prec0$, which holds component-wise, and for any time slot $t$. \label{assum2}
\end{assumption}
\vspace{-1mm}
\noindent This means that there is a Slater vector that satisfies all perturbed instances of (P2). Since the constraints are linear and the perturbations bounded, it is easy to find such a vector (e.g., $y^s=0$). Under this assumption, and given that $f^*$ is bounded, we know that the set of the dual optimal values $\mu^*$ of (D) is bounded, \cite{uzawa}. Now, we define the set:
\begin{equation} 
 Q(\mu_0, \delta_t, \epsilon_t)=\left\{ \mu\geq 0 \mid V(\mu, \delta_t, \epsilon_t)\geq V(\mu_0, \delta_t, \epsilon_t) 	\right\},
\end{equation}
which is parameterized by some dual vector $\mu_0$, and the running averages of perturbations $\delta_t, \epsilon_t$. For every $\mu\in Q(\mu_0, \delta_t, \epsilon_t)$, it holds:
\begin{align}
	V(\mu_0, \delta_t, \epsilon_t)&\leq V(\mu, \delta_t, \epsilon_t) \nonumber \\
	&=\inf_{y\in\mathcal{Y}} \left\{ f(y)+y_t^\top\epsilon_t + \mu^\top\big( g(y)+\delta_t(y) \big) \right\}\nonumber \\
	&\leq f(y^s)+\epsilon_{t}^\top y^s + \sum_{n=1}^{N+1}\mu_n\big( g_n(y^s) + \delta_{nt}(y^s) \big)\Rightarrow \nonumber 
\end{align}
\begin{align}
	& - \sum_{n=1}^{N+1}\mu_n\big( g_n(y^s)+\delta_{nt}(y^s) \big) \leq f(y^s) - V(\mu_0, \delta_t, \epsilon_t)+\epsilon_t^\top y^s
\end{align}
\noindent It is $g_n(y^s)+\delta_{nt}(y^s)<0$, $\mu_n\geq 0$, $\forall n=1,\ldots,N+1$ and $\forall t$, and setting $v=\min_{1\leq n\leq N+1}\{ -g_n(y^s)-\delta_{nt}(y^s) \}$, we can write:
\begin{align}
v\sum_{n=1}^{N+1}\mu_n&\leq -\sum_{n=1}^{N+1}\mu_n\big( g_n(y^s)+\delta_{nt}(y^s)	\big) \nonumber \\
&\leq f(y^s) - V(\mu_0, \delta_t, \epsilon_t)+\epsilon_t^\top y^s,\,\,\,\text{hence} \nonumber \\
\sum_{n=1}^{N+1}\mu_n&\leq \frac{1}{v}\Big( f(y^s)-V(\mu_0, \delta_t, \epsilon_t) +\epsilon_t^\top y^s \Big),
\end{align}
and since $\mu\geq 0$ we have that $\|\mu\| \leq \sum_{n=1}^{N+1}\mu_n$. Therefore:
\begin{equation}
	\max_{\mu \in Q(\mu_0, \delta_t, \epsilon_t)}\|\mu\|\leq \frac{1}{v}\Big( f(y^s) - V(\mu_0, \delta_t, \epsilon_t)+\epsilon_t^\top y^s \Big). \label{eq:34}
\end{equation}

Now, we are going to prove that $\norm{\mu_{t+1}-\mu^*}\leq$
\begin{align}
	&\max\{\norm{\mu_1-\mu^*}, \frac{1}{v}\Big( f(y^s) - V(\mu^*, \delta_t, \epsilon_t) -\epsilon_t^\top y^s \Big) \nonumber \\
	&+\frac{a(\sigma_g+\sigma_{\delta_t})^2 }{2v} + \norm{\mu^*} +a(\sigma_g+\sigma_{\delta_t}) \} \label{eq:11-nedic}
\end{align}
%\ag{Missing $()^2$ in $(\sigma_g+\sigma_{\delta_t})$}
This holds for $t=0$, and we will use induction to prove that it holds for any $t$. We start by expanding the subgradient update:
\begin{align}
	\norm{\mu_{t+1}-\theta }^2 &\leq \norm{ \big[ \mu_t + a\big( g(y_t)+\delta_t(y_t) \big) \big]^+ -\theta  }^2 \nonumber \\
	&\leq \norm{ \mu_t +a\big(g(y_t)+\delta_t(y_t) \big) -\theta }^2 \nonumber \\
	&=\norm{\mu_t-\theta}^2+a^2\norm{g(y_t)+\delta_t(y_t)}^2 + \nonumber \\
	&\quad 2a\big( g(y_t)+\delta_t(y_t)\big)^\top(\mu_t-\theta). \label{eq:35}
\end{align}
Note that $g(y_t)+\delta_t(y_t)$ is a subgradient of $V(\mu_t, \delta_t, \epsilon_t)$. Hence, for any $\theta$, we can write:
\begin{equation}
	\big( g(y_t)+\delta_t(y_t)\big)^\top(\mu_t-\theta)\leq - \big(V(\theta, \delta_t, \epsilon_t)-V(\mu_t, \delta_t, \epsilon_t) \big).
\end{equation}
Replacing this inequality in \eqref{eq:35}, and setting $\theta=\mu^*$, we have:
\begin{align}
	\norm{\mu_{t+1}-\mu^*}^2 &\leq \norm{ \mu_t-\mu^* }^2 + a^2\norm{ g(y_t)+\delta_t(y_t) }^2 - \nonumber \\
	&2a\big( V(\mu^*, \delta_t, \epsilon_t)-V(\mu_t, \delta_t, \epsilon_t) \big) \label{eq:lemma2ned}
\end{align}
As a next step, we bound the distance: 
\begin{align}
	\norm{ \mu_{t+1}-\mu^* } &\leq \norm{ \mu_t +ag(y_t)+a\delta_t(y_t)-\mu^* } \nonumber \\
	&\leq \norm{\mu_t}+\norm{\mu^*}+a\sigma_{g}+a\sigma_{\delta_t}, \label{eq:cases}
\end{align}
%\ag{missing index k in $\mu$ in the above}
where we have used the triangle inequality, and we define the set:
\begin{align}
	&Q(\mu^*, \delta_t, \epsilon_t, a)= \nonumber \\
	&\left\{ \mu\geq 0 \mid V(\mu, \delta_t, \epsilon_t) \geq V(\mu^*, \delta_t, \epsilon_t)-\frac{a(\sigma_{g}+\sigma_{\delta_t})^2}{2} \right\},
\end{align}
which, by definition, is a superset of $Q(\mu^*, \delta_t, \epsilon_t)$. Now, we consider the following two cases. 

\textbf{First case}: $\mu_t$ is such that it belongs to the set $Q(\mu^*, \delta_t, \epsilon_t,a )$. Then, by \eqref{eq:34}, we have: 
\begin{equation}
	\norm{\mu_t}\leq \frac{1}{v}\big( f(y^s)-V(\mu^*, \delta_t, \epsilon_t) +\epsilon_t^\top y^s \big)+\frac{a(\sigma_{g}+\sigma_{\delta_t})^2}{2v},
\end{equation}
which, combined with \eqref{eq:cases}, validates \eqref{eq:11-nedic}. \textbf{Second case}: $\mu_t$ is such that 
\begin{equation}
V(\mu_t, \delta_t, \epsilon_t)<V(\mu^*, \delta_t, \epsilon_t)-\frac{a(\sigma_{g}+\sigma_{\delta_t})^2}{2}.
\end{equation}
From \eqref{eq:lemma2ned} and \eqref{eq:var}:
\begin{align} 
	&\norm{ \mu_{t+1}-\mu^* }^2 \leq \norm{ \mu_t-\mu^* }^2- \nonumber \\
	&2a\Big(V(\mu^*, \delta_t, \epsilon_t)-V(\mu_t, \delta_t, \epsilon_t)-\frac{a(\sigma_{g}+\sigma_{\delta_t})^2}{2} \Big),
\end{align}
where by our assumption the last term is non-positive and can be dropped, thus $\norm{\mu_{t+1}-\mu^*}\leq \norm{ \mu_t-\mu^*}$. Therefore, again we have shown that \eqref{eq:11-nedic} holds by induction for this case as well.

Finally, using \eqref{eq:11-nedic} and $\norm{\mu_1-\mu^*}\leq \norm{\mu_1}+\norm{\mu^*}$, we can write: 
\begin{align}
\norm{\mu_{t+1}}&\leq\norm{ \mu_{t+1}-\mu^* }+ \norm{\mu^*} 2\norm{\mu^*}+\leq \nonumber \\
&\max\Big\{\norm{\mu_1}, \frac{1}{v}\Big( f(y^s) - V(\mu^*, \delta_t, \epsilon_t) -\epsilon_t^\top y^s  \Big) + \nonumber \\
&\frac{a(\sigma_g+\sigma_{\delta_t})^2 }{2v} +a(\sigma_g+\sigma_{\delta_t}) \Big\}, \label{eq:39}
\end{align}
which states that all Lagrange multipliers are upper bounded by constants. To see this, note that: the optimal dual variables $\mu^*$ are bounded; the dual function is bounded for the bounded $\mu^*$ and any combination of perturbations, while we can further set $\mu_1=0$ to simplify the RHS. Since all dual variables are positive, and the norm of the dual vector is bounded, it is clear that the RHS of \eqref{eq:constraint-bound} converges to zero as $T\rightarrow \infty$. Similarly, the second term of the RHS (average value of perturbations) converges to 0, and hence we obtain:
\begin{equation}
	\lim_{T\rightarrow \infty}g(\bar y_T)+\lim_{T\rightarrow \infty}\frac{1}{T}\sum_{i=1}^T\delta_i(y_i) =	\lim_{T\rightarrow \infty}g(\bar y_T)\preceq 0 \nonumber
\end{equation}

Due to the equivalence $\lim_{T\rightarrow\infty}\frac{1}{T}\sum_{t=1}^Tg_{nt}(y_t)=\lim_{T\rightarrow \infty}g_{n}(\bar y_T),\forall n$, we have proved that the \textbf{actual performance and constraint violation} of our system reaches the optimal solution asymptotically.
